# Supplementary material for: Identification of metastable lattice distortion free charge density wave at photoinduced interface via TRARPES
Source: arXiv:2502.06177 source file (2025-02-10)
Supplement: Supplementary file 1 [file SM.pdf]

# Identification of Metastable Lattice Distortion Free Charge Density Wave at Photoinduced Interface via TRARPES

Shaofeng Duan,<sup>1,2</sup> Binshuo Zhang,<sup>3</sup> Zihao Wang,<sup>2</sup> Shichong Wang,<sup>2</sup> Lingxiao Gu,<sup>2</sup> Haoran Liu,<sup>2</sup>  
Jiongyu Huang,<sup>2</sup> Jianzhe Liu,<sup>2</sup> Dong Qian,<sup>2,4,5</sup> Yanfeng Guo,<sup>3,6</sup> and Wentao Zhang<sup>1,2,\*</sup>

<sup>1</sup>Beijing National Laboratory for Condensed Matter Physics,  
Institute of Physics, Chinese Academy of Sciences, Beijing 100190, China.

<sup>2</sup>Key Laboratory of Artificial Structures and Quantum Control (Ministry of Education),  
School of Physics and Astronomy, Shanghai Jiao Tong University, Shanghai 200240, China

<sup>3</sup>School of Physical Science and Technology,  
ShanghaiTech University, Shanghai 201210, China

<sup>4</sup>Tsung-Dao Lee Institute, Shanghai Jiao Tong University, Shanghai 200240, China

<sup>5</sup>Collaborative Innovation Center of Advanced Microstructures,  
Nanjing University, Nanjing 210093, China

<sup>6</sup>ShanghaiTech Laboratory for Topological Physics, Shanghai 201210, China

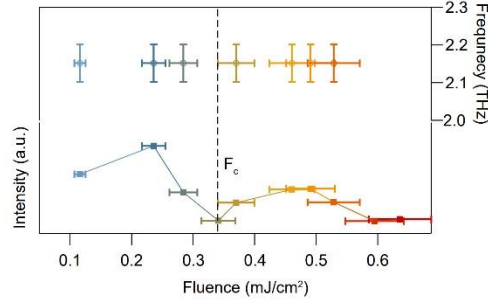

Supplemental FIG. 1. Fluence-dependent frequency (top) and intensity (bottom) of the amplitude mode.

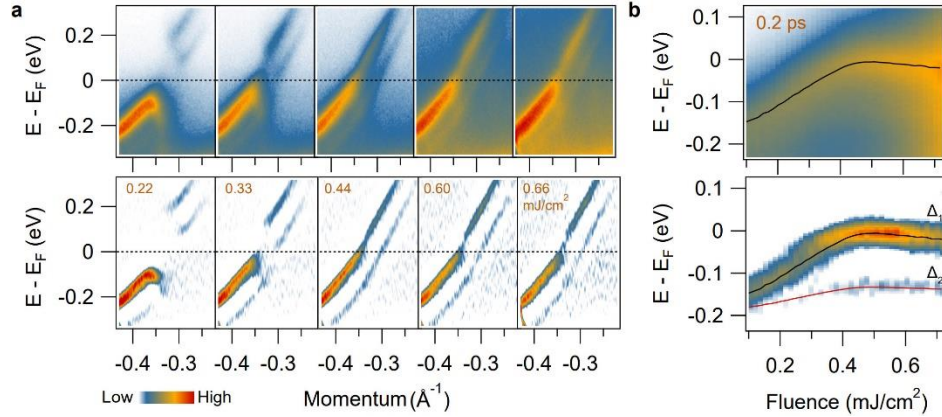

Supplemental FIG. 2. a, Nonequilibrium electronic structures at the delay time of 0.2 ps at selected pump fluence (top) and corresponding second-derivative images along the energy axis (bottom). b, Fluence-dependent photoemission intensity at the Fermi momentum (top) and the corresponding second-derivative image along the energy axis. The black solid lines obtained from Lorentz fitting indicate the peak position of the CDW band ( $\Delta_1$ ), and the red line is rescaled from the peak position of  $\Delta_1$  to track the position of the CDW band  $\Delta_2$ .

\*wentaozhang@iphy.ac.cn

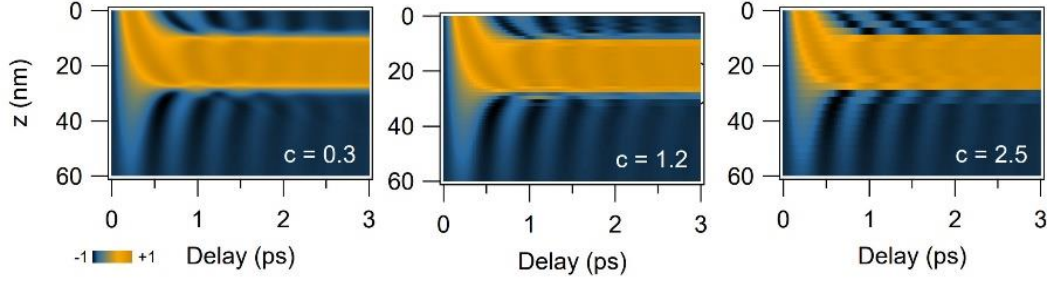

Supplemental FIG. 3. **a**, Order parameters as functions of delay time and depth ( $z$ ) away from the sample surface for selected lattice constants of  $c = 0.3, 1.2$ , and  $2.5$  nm by fixing other parameters  $\tau_e = 0.3$  ps,  $z_p = 20$  nm [S4],  $\omega_0 = 2\pi \cdot 2.15$  THz, and  $\gamma = 0.2$  THz [S5] for  $\text{GdTe}_3$ .

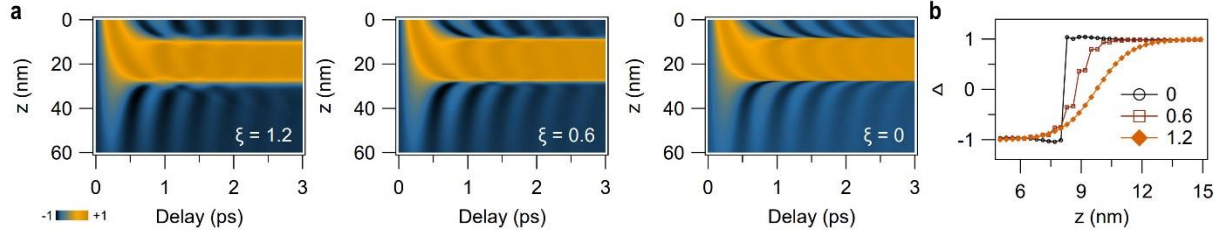

Supplemental FIG. 4. **a**, Order parameters as functions of delay time and depth ( $z$ ) away from the sample surface for selected coherent lengths of  $\xi = 1.2, 0.6$ , and  $0$  nm by fixing parameters  $\tau_e = 0.3$  ps,  $z_p = 20$  nm [S4],  $\omega_0 = 2\pi \cdot 2.15$  THz, and  $\gamma = 0.2$  THz [S5] for  $\text{GdTe}_3$ . **b**, Depth-dependent order parameter at a delay time of 3 ps from panel **a**.

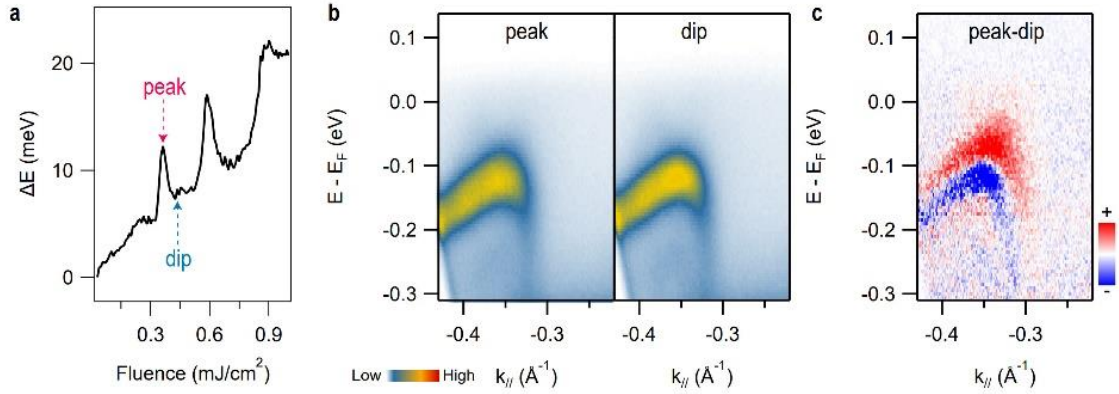

Supplemental FIG. 5. **a**, Fluence-dependent energy shifts of the CDW band at a delay time of 6 ps. The red arrow indicates the fluence for the photoinduced domain boundary placed at the sample surface, and the blue arrow represents the inverted CDW phase. **b**, Transient electronic structures at the fluence of  $0.36$   $\text{mJ}/\text{cm}^2$  (peak: domain boundary) and  $0.42$   $\text{mJ}/\text{cm}^2$  (dip: inverted CDW phase). **c**, The photoemission spectra difference between fluences at peak and dip. The color scale is in arbitrary units, ‘-’ (blue) indicates  $< 0$ , and ‘+’ (red) indicates  $> 0$ .

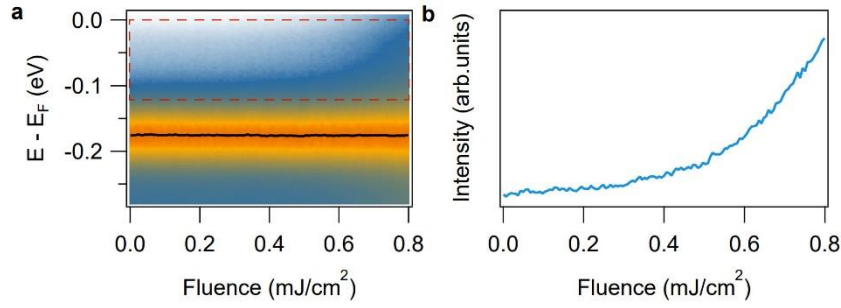

Supplemental FIG. 6. a, Fluence-dependent photoemission intensity at the Fermi momentum (top) at -5 ps. b, fluence-dependent photoemission intensity integrated from  $-0.13$  eV to the Fermi level highlighted by the red dashed box in a.

### Supplementary Note 1

The electronic structure of  $\text{RTe}_3$  can be well described by a simplified tight-binding (TB) model of the Te plane with coupling along ( $t_{\parallel}$ ) and perpendicular ( $t_{\perp}$ ) to the chains, and the spin-orbital couplings were neglected in this calculation [S1-S2]. The dispersion is following this format:

$$E_{p_x}(k_x, k_y) = -2t_{\parallel} * \cos\left[(k_x + k_z) * \frac{a}{2}\right] - 2t_{\perp} * \cos\left[(k_x - k_z) * \frac{a}{2}\right] - E_F$$

$$E_{p_z}(k_x, k_y) = -2t_{\parallel} * \cos\left[(k_x - k_z) * \frac{a}{2}\right] - 2t_{\perp} * \cos\left[(k_x + k_z) * \frac{a}{2}\right] - E_F,$$

where the Fermi level  $E_F = -2t_{\parallel} \sin\left(\frac{\pi}{8}\right)$  was fixed by the band filling. The coupling parameters  $t_{\parallel} \approx -1.9$  eV and  $t_{\perp} \approx -3.5$  eV were adjusted to match the experimental Fermi surface [S1-S2]. The calculated Fermi surface is shown in Fig. 1(b) in the main text, it could well capture the experimental observations with shadow bands and folded bands due to the charge density wave (CDW) phase transitions. The residual spectral intensity at the momentum of  $k_x = 0$  and  $k_z = -0.4 \text{ \AA}^{-1}$  arose from the perpendicular unidirectional CDW domain in  $\text{GdTe}_3$ . Both the domain and bilayer splitting effects were not considered in the calculations.

### Supplementary Note 2

To determine the initial response time of the energy shift after photoexcitation, we perform a Golab fitting of the time-dependent energy shifts. The fitting function takes the form [S3]:

$$E(t) = \left[ \frac{A_0}{2} \left( 1 + \text{Erf}\left(\frac{2\sqrt{2}(t-t_0)}{w_1}\right) \right) * \left( A_1 e^{\left(\frac{-t-t_0}{\tau_1}\right)} + A_2 e^{\left(\frac{-t-t_0}{\tau_2}\right)} \right) \right] * g(w_0, t),$$

where  $w_1$  denotes the full width at half maximum of the intrinsic response time after photoexcitation,  $t_0$  is the time delay for the energy shifts rising to half of its maximum value,  $A_0$  signifies the photoinduced maximum energy shift,  $A_1$  and  $A_2$  indicating the amplitudes of the dual-stage decay process of the energy shifts, and  $\tau_1$  and  $\tau_2$  representing the relaxation times for the faster and slower decay process, respectively. Additionally, the rising time of the photoinduced energy shift is also limited by the time resolution of the instrument. A normalized Gaussian function representing the time resolution of the TRARPES system was convolved with the terms in the square brackets.

### Supplementary Note 3

In the case of a damped oscillation, the oscillation frequency of the system decreases as the damping

coefficient ( $\beta$ ) increases by  $\sqrt{\omega_0^2 - \beta^2}$ , ultimately vanishing in the overdamped regime. In contrast to the reduced frequency typically observed in such overdamped scenarios, the oscillation frequency of the CDW-coupled amplitude mode disappeared at the critical pump fluence without showing any frequency softening during the photoinduced transition in GdTe<sub>3</sub> (Supplemental FIG. 1). Instead, the oscillation frequency remains nearly independent of fluence both below and above the CDW melting threshold (Figs. 2(c) and (d), and Supplemental FIG. 1), deviating from the typical behavior expected in the overdamped picture. The absence of coherent oscillations, combined with the lack of frequency softening across in the transition, provides strong evidence for the absence of lattice distortions in the photoinduced interface CDW state.

#### Supplementary Note 4

With optical excitation, multi-photon absorption processes become significant at higher pump fluence, enabling electrons below the Fermi level to simultaneously absorb the energy of two or more photons, leading to their emission from the material. Photoelectrons generated through the multiphoton absorption process do not provide intrinsic information on the electronic states of the material, as their energy and momentum distributions are determined by the nonlinear effects of the pump fluence. The multi-photon absorption processes result in a broad and unstructured energy distribution signal at higher pump fluences and this background signal becomes significant in the measured energy and momentum window as the pump fluence increases, shown in the fluence-dependent electronic structure at 0.2 ps in Supplemental FIG. 2a at higher pump fluences. In addition, the multi-photon effect could be visualized from the time-dependent photoemission intensity at delay time -5 ps, we found the intensity of the background becomes visible by increasing the pump fluence (Supplemental FIG. 6b).

#### Supplementary Note 5

In GdTe<sub>3</sub>, the CDW transition is primarily driven by Fermi surface nesting, which serves as a unified mechanism for the formation of the two CDW gaps. While these gaps differ in magnitude below the Fermi energy, their common origin suggests that they should exhibit a consistent response following ultrafast optical excitation. This is supported by our observations in the fluence-dependent photoemission intensity near the Fermi momentum at 0.2 ps, where the two CDW gaps associated with the bilayer splitting exhibit a similar response and were simultaneously suppressed within 0.2 ps after photoexcitation above a specific pump fluence (Fig. 3a and Supplemental FIG. 2a). The black solid line in Supplemental FIG. 2b shows the peak position of the CDW band with an energy gap of  $\Delta_1$ , derived from Lorentz function fitting. However, the weaker photoemission intensity of the CDW band with  $\Delta_2$  makes it challenging to determine its peak position through fitting. To better track the peak position of the CDW band with  $\Delta_2$ , we rescale the energy shifts of the CDW band with  $\Delta_1$  by applying a scale factor. The resulting rescaled curve aligns with the energy shifts of the CDW band with  $\Delta_2$  (red line in Supplemental FIG. 2b). As the pump fluence increases, both gaps decrease and exhibit a plateau above a certain excitation level, indicating a common origin for these two gaps

#### Supplementary Note 6

The free energy  $V$  as a function of the order parameter  $\Phi$ , depth  $z$  away from the sample surface, and time  $t$  is given by:

$$V(\Phi, z, t) = \frac{1}{4}(\eta(t) - 1)\Phi^2 + \frac{1}{8}\Phi^4 + \frac{1}{4}\xi^2 \left(\frac{\partial \Phi}{\partial z}\right)^2,$$

where  $\xi$  is the coherence length,  $\eta(t) = \eta_0 e^{(-t/\tau_e)} e^{(-z/z_p)}$  represents the transient modification of the Landau potential with excitation density  $\eta_0$ ,  $\tau_e$  is the nonequilibrium quasiparticle decay rate, and  $z_p$  is the penetration depth of the incident laser.

The corresponding equation of motion for the order parameter after photoexcitation is:

$$\frac{1}{\omega_0^2} \frac{\partial^2}{\partial t^2} \Phi + \frac{\gamma}{\omega_0} \frac{\partial}{\partial t} \Phi - \frac{1}{2} (1 - \eta(t)) \Phi + \frac{1}{2} \Phi^3 - \frac{\xi^2}{2} \frac{\partial^2}{\partial z^2} \Phi = 0,$$

where  $\omega_0$  is the angular frequency of the collective amplitude mode responsible for CDW formation, and  $\gamma$  is the damping coefficient for the amplitude mode. The ultrafast dynamics and spatial distributions of the order parameter in the main text can be numerically solved based on this motion equation with parameters  $\xi = 1.2$  nm [S4-S5],  $\tau_e = 0.3$  ps,  $z_p = 20$  nm [S4],  $\omega_0 = 2 * \pi * 2.15$  THz, and  $\gamma = 0.2$  THz [S5] in GdTe<sub>3</sub>, and numerical solutions of the motion equation are described in Ref. [S6]

### Supplementary Note 7

According to the universal curve of electron escape depth as a function of electron kinetic energy, the mean free path of electrons for the 6 eV photons used in our experiments is approximately 3 nm. This depth, closely matching the lattice constant of 2.56 nm along the direction perpendicular to the cleaving surface in GdTe<sub>3</sub>, ensures that the measured photoemission spectrum predominantly reflects electronic structures at the surface. In addition, given a penetration depth of 20 nm for the infrared pump laser, the estimated depth corresponding to the absorption of the pump pulse energy within the peak range in the fluence-dependent energy shifts is approximately 2.67 nm, comparable to the lattice constant of 2.528 nm, indicating that the photoinduced interface may be confined within a single unit cell.

The above findings are further supported by simulations, and we performed detailed calculations by altering the lattice constant perpendicular to the sample surface (Supplemental FIG. 3) as well as the coherent length of the CDW order (Supplemental FIG. 4) to elucidate their impacts on the characteristics of the photoinduced domain walls. The simulations demonstrate that for the same pump fluence, sharper domain walls are obtained with an increase in the lattice constant perpendicular to the sample surface, and for a larger lattice constant of 2.5 nm, the photoinduced domain wall was nearly confined within a single-layer unit cell (Supplemental FIG. 3). Furthermore, the photoinduced domain walls exhibit narrower intervals between the order parameter  $\Phi = -1$  and  $+1$  when the coherent length of the CDW order is reduced (Supplemental FIG. 4). Consequently, it is possible to realize domain walls with distinct properties in different materials by varying factors such as the lattice constant, coherent length, and others.

The close alignment between the probing depth (3 nm) of the 6 eV photon, the estimated thickness of the photoinduced domain interface (2.67 nm), and the lattice constant (2.528 nm) enable effective investigation of the interface CDW state within one unit cell when the interface is positioned at the sample surface at specific pump fluence while minimizing bulk contributions. Therefore, the observed gap opening and the lattice distortion-free dynamics in our manuscript could be regarded as the characteristic features of the photoinduced interface CDW state.

### Supplementary Note 8

The Fermi surface of the photoinduced interface CDW state possibly exhibits a distinct electronic structure compared to the initial or inverted state, such as the modified CDW nesting vector. By closely examining the electronic structures at the photoinduced domain boundary (peak) and inverted CDW states (dip), we found that the gap at the photoinduced domain boundary is smaller than in the inverted CDW phase. As depicted in Supplemental FIG. 5, the CDW gap at the photoinduced domain boundary is only a few meV smaller than that of the inverted phase. With the CDW gap being approximately 170 meV in equilibrium, such a minor gap variation is difficult to discern from the raw E-K images (Supplemental FIG. 5b). However, the change in gap size is evident in the intensity of the photoelectron spectrum. The spectral difference between the domain boundary and the inverted CDW state reveals a further increment in spectral intensity within the CDW gap (Supplemental FIG. 5c), indicating that the CDW gap at the photoinduced domain

boundary is reduced and smaller than the bulk, even at a smaller pump fluence. The absence of the CDW-coupled amplitude mode in the time-resolved electronic structure at the domain boundary suggests the presence of a new phase without lattice distortions. Thus, we associate the photoinduced domain boundary with an exotic interface CDW state characterized by a reduced gap and absence of lattice distortions in our manuscript.

## Supplementary Note 9

In time-resolved ARPES experiments, the photoinduced thermal effects can become particularly significant when the sample is exposed to pump laser pulses with high repetition rates. Once the sample is excited, the system may not fully return to its equilibrium state before the arrival of the next pump pulse, resulting in cumulative heating and overheating of the sample in some materials. This overheating can induce extrinsic effects in the experiments, such as the spectral broadening and noticeable energy shifts in the electronic structure as the pump fluence increases. The repetition rate of the pump laser is set to 500 kHz, resulting in a 2  $\mu$ s interval between consecutive pump pulses. This interval is several orders of magnitude longer than the typical relaxation time of the photoinduced hot electrons, which ranges from tens to hundreds of picoseconds. To eliminate the influence of photoinduced thermal effects and verify the system returned to its equilibrium state between two consecutive pump pulses in the time-resolved ARPES experiments, we performed fluence-dependent measurements of the electronic structure at a delay time of -5 ps before conducting detailed time- and fluence-dependent electronic measurements on each sample. The electronic structure of the CDW band at delay times of -5 ps remains unaffected, showing no obvious energy shifts and spectral broadening as the pump fluence increases (Supplemental FIG. 6a), indicating that the steady-state thermal effect induced by the pump laser pulses is negligible in our time-resolved ARPES experiments. The enhanced background at high pump fluence is a result of the multiphoton photoemission effect induced by the pump.

- [S1] V. Brouet, W. L. Yang, X. J. Zhou, Z. Hussain, R. G. Moore, R. He, D. H. Lu, Z. X. Shen, J. Laverock, S. B. Dugdale, N. Ru, and I. R. Fisher, Angle-resolved photoemission study of the evolution of band structure and charge density wave properties in  $R\text{Te}_3$  ( $R = \text{Y, La, Ce, Sm, Gd, Tb, and Dy}$ ), *Phys. Rev. B* 77, 235104 (2008).
- [S2] L. Rettig, R. Cortés, J.-H. Chu, I. R. Fisher, F. Schmitt, R. G. Moore, Z.-X. Shen, P. S. Kirchmann, M. Wolf, and U. Bovensiepen, Persistent order due to transiently enhanced nesting in an electronically excited charge density wave, *Nat. Commun.* 7, 10459 (2016).
- [S3] A. Zong, A. Kogar, Y.-Q. Bie, T. Rohwer, C. Lee, E. Baldini, E. Ergecen, M. B. Yilmaz, B. Freelon, E. J. Sie, H. Zhou, J. Straquadine, P. Walmsley, P. E. Dolgirev, A. V. Rozhkov, I. R. Fisher, P. Jarillo-Herrero, B. V. Fine, and N. Gedik, Evidence for topological defects in a photoinduced phase transition, *Nat. Phys.* 15, 27 (2019).
- [S4] M. Trigo, P. Giraldo-Gallo, J. N. Clark, M. E. Kozina, T. Henighan, M. P. Jiang, M. Chollet, I. R. Fisher, J. M. Glowia, T. Katayama, P. S. Kirchmann, D. Leuenberger, H. Liu, D. A. Reis, Z. X. Shen, and D. Zhu, Ultrafast formation of domain walls of a charge density wave in  $\text{SmTe}_3$ , *Phys. Rev. B* 103, 054109 (2021).
- [S5] R. Yuzupov, T. Mertelj, V. V. Kabanov, S. Brazovskii, P. Kusar, J.-H. Chu, I. R. Fisher, and D. Mihailovic, Coherent dynamics of macroscopic electronic order through a symmetry breaking transition, *Nat. Phys.* 6, 681 (2010).
- [S6] S. Duan, Y. Cheng, W. Xia, Y. Yang, C. Xu, F. Qi, C. Huang, T. Tang, Y. Guo, W. Luo, D. Qian, D.

Xiang, J. Zhang, and W. Zhang, Optical manipulation of electronic dimensionality in a quantum Material, Nature 595, 239 (2021).
